# Supplementary material for: Search for synchrotron emission from secondary electrons of proton-proton interaction in Galactic PeVatron candidate HESS J1641$-$463
Source: arXiv:2404.11012 source file (2024-04-17)
Supplement: Supplementary file 1 [file appendix.tex]

%%%%%%%%%%%%%%%%%%%%%%%%%
%%%%%%%%%%%%%%%%%%%%%%%%%
\clearpage

\appendix

\section{\nustar\ analysis with nuskybgd} 
\label{sec:nuskybgd}
%%%%%%%%%%%%%%%%%%%%%%%%%
%%%%%%%%%%%%%%%%%%%%%%%%%

\begin{figure}[ht!]
\plotone{nuskybgd_image.png}
\caption{
Regions for nuskybgd analysis.
\label{fig:nuskybgd_image} }
\end{figure}

\subsection{Leptonic scenario} \label{sec:leptonic}
%%%%%%%%%%%%%%%%%%%%%%%%%
%%%%%%%%%%%%%%%%%%%%%%%%%
\comment{move to Discussion part}

%%% Model
The leptonic-dominated model consists of \ac{ic} scattering and synchrotron radiation from primary \ac{cr} electrons.
Spectrum of the primary electrons is assumed to be power-law with an exponential cutoff, given by \eqref{eq:proton}.
CMB, NIR, and FIR are included for calculation of \ac{ic} as seed photon fields, assuming typical values (i.e., temperatures of 2.72 K, 30 K, and 3000 K, and energy densities of 0.261, 0.5, and 1 eV~cm$^{-3}$, respectively).
\check{check how different the photon fields are around \j1641}
%These values are adopted for the photon field throughout this paper.

%%% cooling
%Here, we do not solve time evolution due to radiation cooling.
Because the TeV gamma-ray flux is compatible with the X-ray upper limits, $B \sim 3$ \uG\ \check{} in the leptonic model.
With such low magnetic field, cooling (due to synchrotron radiation) is not effective, and the spectrum of electrons is not largely modified by the radiation cooling.

%%% fit gamma-ray; Model 1--3: 
First, we fit the TeV gamma-ray spectrum with an electron index ($s_e$) free (referred to as Model 1) and fixed to 2 and 3 (Models 2 and 3, respectively).
All the models are summarized in \tabref{tab:leptonic}, and the \acp{sed} are illustrated in \figref{fig:leptonic}.
With the index being free (Model 1), $s_e$ was obtained to be $2.6 \pm 0.2$, but the cutoff energy ($E_{c,e}$) was hardly constrained.
Models 2 and 3 yeilded $E_{c,e}$ of $>$50 TeV and $>$1000 TeV, respectively.
Second, we added the synchrotron radiation from the same electrons not to exceed the observed X-ray upper limits, resulting in $B<$2--3 \uG\ in Models 1--3.
It should be noted that Models 1--3 cannot reproduce the radio observation (\figref{fig:leptonic}).

%%% fit MWL SED; Model 4: 
We also performed a fitting of multiwavelength \ac{sed}, including the radio, X-ray, and TeV gamma-ray data, with $s_e$ being free (Model 4; \tabref{tab:leptonic} and \figref{fig:leptonic}).
The spectral index and magnetic field were respectively estimated to be $2.9 \pm 0.1$ and $2.5^{+0.8}_{-0.5}$ \uG, while the cutoff energy was poorly determined, $E_{c,e} > 200$ TeV.

%%% 
\comment{move to Discussion part?}
In all cases (Models 1--4), the magnetic field should be less than $\sim$3 \uG, which is comparable to the typical value of the interstellar magnetic field, implying that
no shock compression and/or amplification are required.
% We
The electron total energy ($W_e$) was (1--5)$\times 10^{47}$ erg for Models 1--3. \check{add comments on We}

conclusion: leptonic-dominated case is disfavored, although it is not excluded\check{}

\check{check how much reliable the radio data is}

\check{the TeV gamma-ray spectrum is a bit steeper in \cite{HESS2018_HGPS}. If we adopt the steep one, how the result/conclusion changes}

% ===========================
\begin{figure}[ht!]
\centering
%\plotone{sed_leptonic.png}
%\includegraphics[width=0.6\linewidth]{figures/sed_leptonic.png}
\includegraphics[width=0.6\linewidth]{figures/J1641_leptonic_paper.pdf}
\caption{
SED modeling in the leptonic case.
%\check{Add IC models with $s=2,~ 3$, and remove synchrotron models except for $B=2$\uG. }
\label{fig:leptonic} }
\end{figure}
% ===========================

% ===========================
\begin{deluxetable}{ llllll }[ht!]
\tablecaption{
Leptonic models
\label{tab:leptonic}
}
\tablewidth{0pt}
\tablehead{
\colhead{Model} & \colhead{} & \colhead{ 1 } & \colhead{2 } & \colhead{ 3 } & \colhead{ 4 }
}
\startdata
%Ambient density & $n$ & 100 \cc \\
%Distance & $d$ & 11 kpc \\
%Age & $T$ & 5 kyr \\
Electron spectral index & $s_e$                 & $2.6 \pm 0.2$   & 2 (fixed)   & 3 (fixed)   & $2.9\pm 0.1$ \\
Electron cutoff energy  & $E_{c,e}$ (TeV)       & not constrained        & $>$50        & $>$1000        & $>$200 \\
Electron total energy   & $W_e~ (E>1$TeV) ($10^{47}$ erg) &  2.5 &  1.1 &  4.5 &  $3.6 \pm 0.6 $ \\
Magnetic field          & $B$ (\uG )            & $<$2    & $<$2    & $<$3    & 2.5$^{+0.8}_{-0.5}$ \\
Note & & \multicolumn{3}{c}{Fit gamma-ray and add synchrotron} & MWL fitting \\
\enddata
\tablecomments{
Table notes.
}
\end{deluxetable}
% ===========================
